# Supplementary material for: Efficient All-to-All Collective Communication Schedules for Direct-Connect Topologies
Source: arXiv:2309.13541 source file (2024-04-25)
Supplement: Supplementary file 1 [file supplemental.tex]

\appendix
\section{Upper Bound for \ata Performance}\label{sec:ub_proof}
Proof of Theorem 1 (Main paper).
\begin{proof}
	For any flow from $s$ to $t$, we can decompose it to paths $p_1,\dots,p_n$ and $f_1,\dots,f_n$ such that $p_i$ delivers $f_i$ amount of flow from $s$ to $t$. Note that $\sum_i f_i=f$ and $\ell(p_i)\geq d(s,t)$. The cost of capacity for this flow is
	\[
		\sum_{i=1}^n f_i\cdot\ell(p_i)\geq\sum_{i=1}^n f_i\cdot d(s,t)=f\cdot d(s,t).
	\]
\end{proof}

\noindent Proof of Theorem 2 (Main paper).
\begin{proof}
	Consider a single-source multicommodity flow, where the source needs to send $N-1$ flows to the other $N-1$ destinations. Since the network is $d$-regular, there are at most $d^k$ nodes at exactly distance $k$ from the source. Thus, the optimal network for single-source multicommodity flow is $T(d,N)$, and the minimum cost of capacity is $f\cdot\tau(d,N)$. It immediately follows that the minimum cost of capacity for all-source multicommodity flow is $N\cdot f\cdot\tau(d,N)$. Because the total capacity of the network $G$ is $d\cdot N$ (assuming capacity $1$ at each edge), we have $N\cdot f\cdot\tau(d,N)\leq d\cdot N$, and the inequality trivially follows.
\end{proof}

\section{Additional evaluation results}

Figure~\ref{fig:torusperf-xml} compares the performance of tsMCF with ompi/ oneCCL baseline on the $3 \times 3$ torus on TACC. Although the network cards are capable of forwarding, they do not have any additional bandwidth because the host-to-NIC bandwidth matches the total NIC egress/ingress bandwidth. In this scenario, our optimized tsMCF schedules yield $66\%$ higher throughput compared to the baseline.  

Figure~\ref{fig:genkautz_vs_lb_d8_16} shows the simulated throughput performance of Generalized Kautz for degree $d=8,16$. We observe that the throughput performance of Generalized Kautz remains close to the lower bound on optimal all-to-all time at large degrees. Figure~\ref{fig:genkautz_d6} shows that the MCF throughput on Generalized Kautz is about $~10\%$ higher compared to other expander topologies at $d=6$.

In Figure~\ref{fig:host_to_nic} we vary the importance of topology in the presence of host-to-nic bottlenecks. We simulate a degree 4 network with egress bandwidth out of a NIC = 4, and then we sweep the host-to-nic bandwidth from 4 (no bottleneck) downwards to 0.5 (severe bottleneck). We observe that expander graphs (GenKautz and Shortest path expanders (see Section \ref{sec:incspath})) yield high \ata performance compared to same sized tori until a certain degree of the bottleneck (around 1.3). For even greater degrees of the host-to-nic bottleneck, the advantage of expanders is erased and the 10x10 torus starts performing equally well.

\begin{figure}
\centering
\includegraphics[scale=0.45]{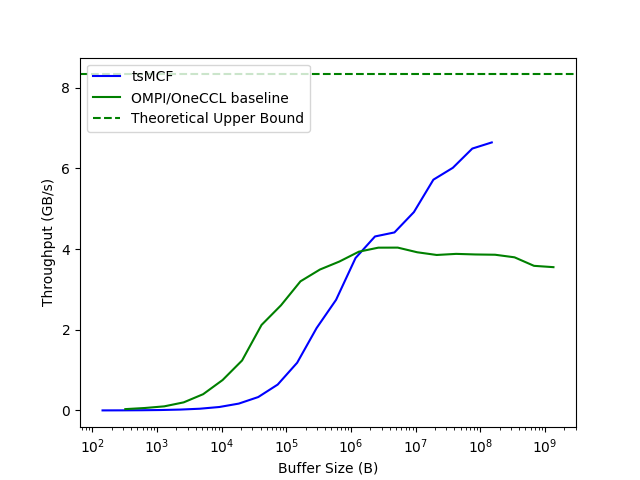}
\caption{Performance of lowered all-to-all link-based schedules on 2-D Torus (TACC testbed).}
\label{fig:torusperf-xml}
\end{figure}

\begin{figure}
\centering
\includegraphics[scale=0.55]{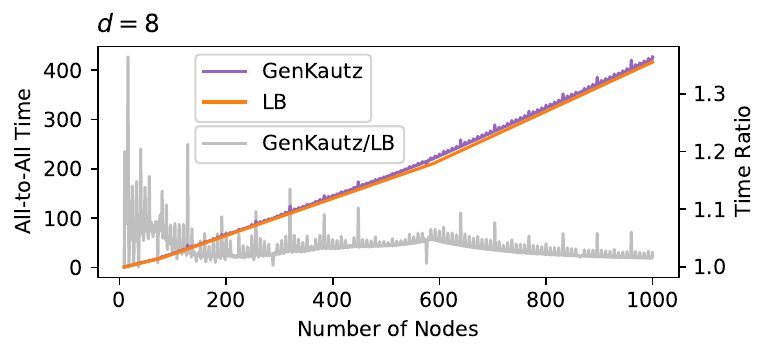}
\includegraphics[scale=0.55]{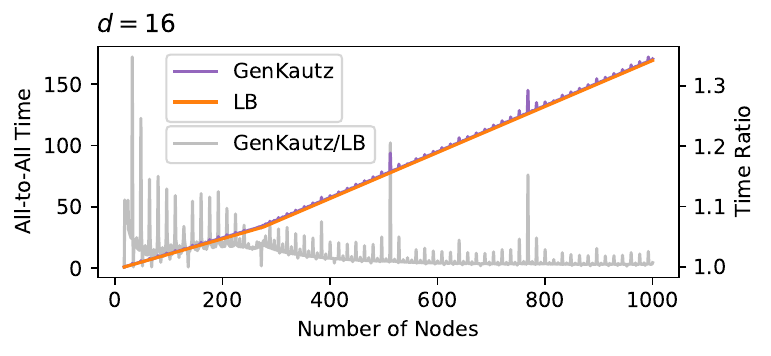}
\caption{Performance of Generalized Kautz graph with respect to the alltoall lower bound for varying graph size ($N$ upto $1000$ nodes) and degree $d=8,16$.}
\label{fig:genkautz_vs_lb_d8_16}
\end{figure}

\begin{figure}
\centering
\includegraphics[scale=0.45]{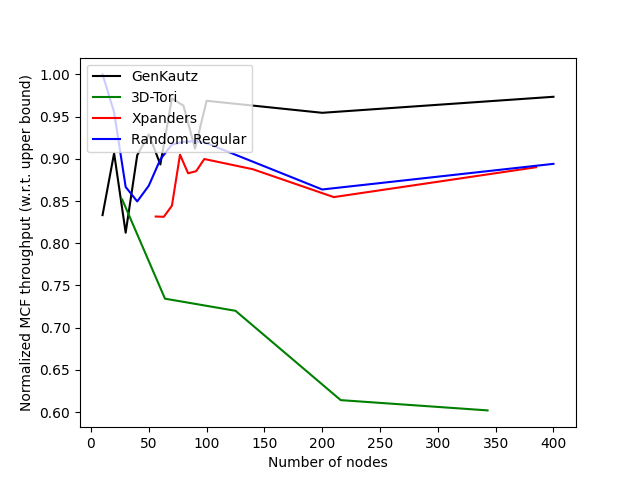}
\caption{Performance of Generalized Kautz graph relative to well-known expander topologies for varying graph size ($N$ upto $400$ nodes) and $d=6$}
\label{fig:genkautz_d6}
\end{figure}

\begin{figure}
\centering
\includegraphics[width=0.8\columnwidth]{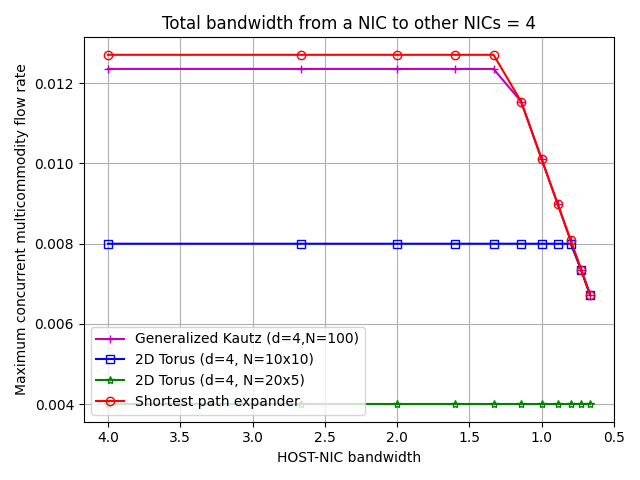}
\caption{Optimal MCF rate for expander graphs and 2D tori as Host-to-NIC bandwidth becomes a bottleneck}
\label{fig:host_to_nic}
\end{figure}

\section{Matrix representation of MCF}

The link-based MCF formulation described in Section 3.1.1 (Main paper) can also be represented in a matrix-vector form. Compactly represented matrix-vector formulations are efficient for LP solvers in contrast to per-edge based summation formulations, since the pre-solve step of constructing the canonical matrix form from a given set of linear constraints can be completely eliminated. This is possible for problems such as MCF since they involve natural matrices like the incidence matrix of a graph that encode the structure of the network as well as flow conservation constraints. This re-formulation has a significant impact on the solution time for large problems involving several hundreds to thousands of nodes. 

The incidence matrix of digraph $G$ is an $N\times |E|$ dimensional matrix $\mathbf{M}$ where $e=(u,v)$, $\mathbf{M}_{u,e}=-1$ and $\mathbf{M}_{v,e}=1$. Define a $|E|\times N(N-1)$ dimensional flow matrix variable $\mathbf{f}$, where entry $\mathbf{f}_{e,c}\in\mathbb{R}_{\geq 0}$ denotes the amount of flow of commodity $c\in \mathcal{C}$ transmitted on link $e\in G$. Denote the link capacities by a $|E|$ dimensional vector $\mathbf{r}$. Additionally, define a scalar variable $F \in \mathbb{R}_{\geq 0}$ denoting concurrent demand, which we want to maximize. The uniform demand matrix corresponding to alltoall multicommodity flow is represented by the $N\times N(N-1)$ dimensional matrix $\mathbf{D}$ where for commodity $c\equiv (s,d) \in \mathcal{C}$, $\mathbf{D}_{s,c}=-1$ and $\mathbf{D}_{t,c}=1$. 

The optimization problem is stated below.

\begin{small}
\begin{center}
\noindent\textbf{\underline{Link-based MCF (compact matrix representation)}}
\end{center}
\begin{align}
&\mbox{maximize }  F \label{eq:mcmcf-matrix-F} \\
&\mbox{subject to:}\notag\\
&\mathbf{f}\:\mathbf{1} \leq \: \mathbf{r} \quad \textrm{(link capacity constraint)} \label{ineq:mcmcf-matrix-capacity} \\
&\mathbf{M}\:\mathbf{f} = \:F\:\mathbf{D} \quad \textrm{(flow \& demand conservation)} \label{ineq:mcmcf-matrix-flow-conservation} \\
&\mathbf{f} \geq \:0 \quad \textrm{(non-negativity of flow)} \label{ineq:mcmcf-matrix-non-negativity}
\end{align}
\end{small}
where $\mathbf{1}$ is a $N(N-1)$ dimensional vector if all 1's.

\section{Achieving \ata\! via unweighted paths}
\label{sec:pathfabric}

Certain network fabrics, e.g., Rockport NIC, that support source routing do not offer native support for weighted routing of commodities along a static set of paths where the weights on various paths may be unequal. We therefore consider the problem where each commodity can be spread along a fixed set of static paths (with the same cardinality, $k$). In particular, we consider the simplest case of this problem where each commodity follows exactly one path, i.e., $k=1$. Under such constraints, the goal of minimizing completion time for the \ata\! workload boils down to choosing $N(N-1)$ distinct paths, one for each commodity, such that the maximum number of paths passing through any link in the network is minimized. This is because the \emph{bottleneck} link in the network will govern the completion rate for the workload. Suppose the bottleneck link $\ell$ in the network has $n_\ell$ paths passing through it and carrying their respective commodities. If all links have link capacity 1, then the rate at which each commodity passing through $\ell$ will be served is proportional to $\frac{1}{n_\ell}$ and hence the time to completion is proportional to $\frac{1}{\frac{1}{n_\ell}} = n_\ell$. Since all commodities want to finish concurrently and we want to minimize the completion time, our goal is to minimize $n_\ell$.

We formulate this optimization problem using Integer Linear Programming (ILP) starting from a set of $(s,d)$ paths like in Section 3.1.4 (Main paper). First, compute the set of paths ${\mathcal P}$ for each commodity (i.e., every pair of nodes). Although ${\mathcal P}$ can be exponentially large, we sample a polynomial size subset, e.g., a set of all disjoint paths. Next, for each path $p\in {\mathcal P}$, define an indicator variable (i.e., 0/1 integer variable) $x_p \in \{0,1\}$, denoted in vector notation as $\mathbf{x}$. Also, define an integer variable $d\in \mathbb{Z}^+$.
For each $p\in {\mathcal P}$ such that $p = (e_1, e_2, \cdots, e_{|p|-1})$, define link-to-path incidence matrix $\mathbf{M}$ such that $\mathbf{M}[e_i][p] = 1$. The dimensionality of $\mathbf{M}$ is $|E|\times |{\mathcal P}|$.
Define a commodity-path incidence matrix $\mathbf{Q}$ such that $\mathbf{Q}_{(s,d),p} = 1$ if path $p$ carries commodity $(s,d)$. The dimensionality of $\mathbf{Q}$ is $N(N-1)\times |{\mathcal P}|$.

The ILP formulation is stated below.\\

\begin{small}
\begin{center}
\noindent\textbf{\underline{Minimum Edge Congestion Routing (ILP)}}\\
\emph{(for equal weight routing on source-routed fabrics)}
\end{center}
\vspace{-2ex}
\begin{align}
&\mbox{minimize }  d \label{eq:path-ILP} \\
&\mbox{subject to:}\notag\\
&\mathbf{M}\:\mathbf{x} \leq d\:\mathbf{1}_{|E|}\label{ineq:path-ilp-maxload}\\
&\mathbf{Q}\:\mathbf{x} = \mathbf{1}_{N(N-1)}\label{eq:path-ilp-uniquepathcomm}\\
&\mathbf{x} \in \{0,1\}^{|{\mathcal P}|}\\
&d \in \mathbb{Z}^+
\end{align}
\end{small}

Inequality \eqref{ineq:path-ilp-maxload} captures the fact that the maximum load (number of commodity carrying paths) passing through any link in the network is $d$, and equation \eqref{eq:path-ilp-uniquepathcomm} ensures that each commodity is carried by exactly one path.

Our analysis shows that the above ILP scheme can match the MCF throughput using a single path per commodity for $3\times 3$ and $3\times 3\times 3$ torus networks. For larger networks, solving ILPs become challenging. For example, for $3\times 3\times 3\times 3$ torus, it does not produce a good solution even in an hour. In general, ILP based solutions do not scale to hundreds of nodes. To deal with this challenge, we adopt heuristic approaches described below inspired by the SSSP heuristic~\cite{Domke11}:
\begin{enumerate}
\item Pass a tolerance factor $\alpha$ to the MILP solver, e.g., Gurobi, Mosek, etc., so that the solver terminates when it has found a solution within $1+\alpha$ factor of the lower bound obtained by LP relaxation.
\item Develop heuristic algorithms based on graph theoretic insights. We developed a greedy algorithm called \texttt{Load aware shortest path} that heuristically minimizes the maximum load on a link as follows:
\begin{enumerate}
\item Start with a graph $G$ where each link has weight $N^2$. (the weight is set to a value greater than the number of commodities, so that the order in which the commodities are routed do not affect the routes~\cite{Domke11})
\item Pick a random $(s,d)$ pair and compute a shortest path $p$ between them.
\item For all links along $p$, increase the link weight by 1.
\item Repeat the last 2 steps until we have routed all commodities.
\end{enumerate}
\end{enumerate}

The \texttt{Load aware shortest path} algorithm scales to large networks but it significantly underperforms MCF, or ILP in cases where the latter is tractable (by more than 2x). Nevertheless, if one wants a set of simple paths for routing the \ata\! collective in a source routed fabric, it is a reasonable heuristic choice.

\subsection{Avoiding deadlocks in wormhole routed fabrics}

In direct connect fabrics that use wormhole routing (or flit-based routing) such as Rockport NICs, avoiding deadlocks is a key concern. This is because when the ILP-generated routes are lowered, the corresponding transmissions occur on shared channels with induced dependencies among them. With the \ata\! traffic pattern, the probability of the occurrence of a cycle in the channel dependency graph increases, and with a high enough load this cycle actually becomes operative and we enter a deadlocked state.

A common prescription to breaking deadlocks is to use virtual channels (VC) and map different operations to different VCs such that there is no cyclic dependency on any of the VCs~\cite{dally1987deadlock}. If the number of VCs is high, then preventing cyclic dependencies is not difficult. However if the number of VCs is low, then doing this needs more careful thinking.

We implemented the following heuristic methods to avoid deadlocks by starting from different sets of high performance routes (per MCF or ILP simulation) and assigning VCs to them algorithmically to be able to lower the routes on the source routed Rockport network:
\begin{enumerate}
\item \textbf{Breaking cycles:} Examine the cycles in a VC dependency graph on a single channel and then break each cycle by assigning alternate VCs to a subset of the links, while taking care that new cycles do not emerge as a result of this process. If they do, then remove cycles iteratively until there are no more of them.
\item \textbf{Random VC assignment:} For a given set of routes (say generated by an ILP or by a greedy heuristic), randomly assign each route one-by-one to a VC that has low usage on or around the links that are part of the current route.
\item \textbf{Algorithmic VC assignment:} For a given set of generated routes and a given number of VCs, perform algorithmic channel assignment on an appropriate conflict graph such that it leads to no cycles. This can be done iteratively.
\end{enumerate}

\begin{figure*}[ht!]
\centering
\includegraphics[width=0.27\textwidth]{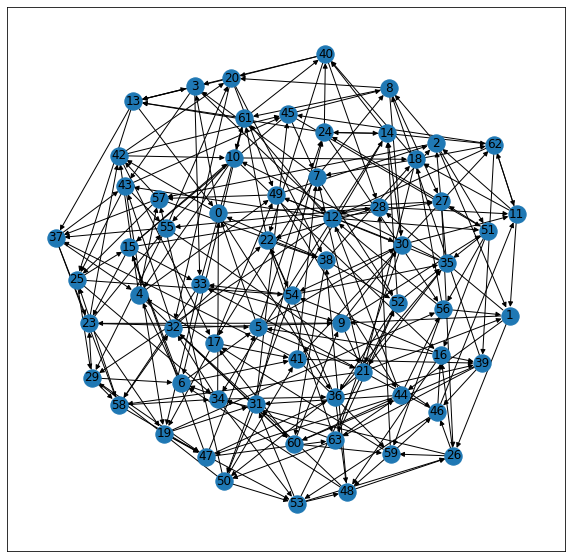}
\includegraphics[width=0.3\textwidth]{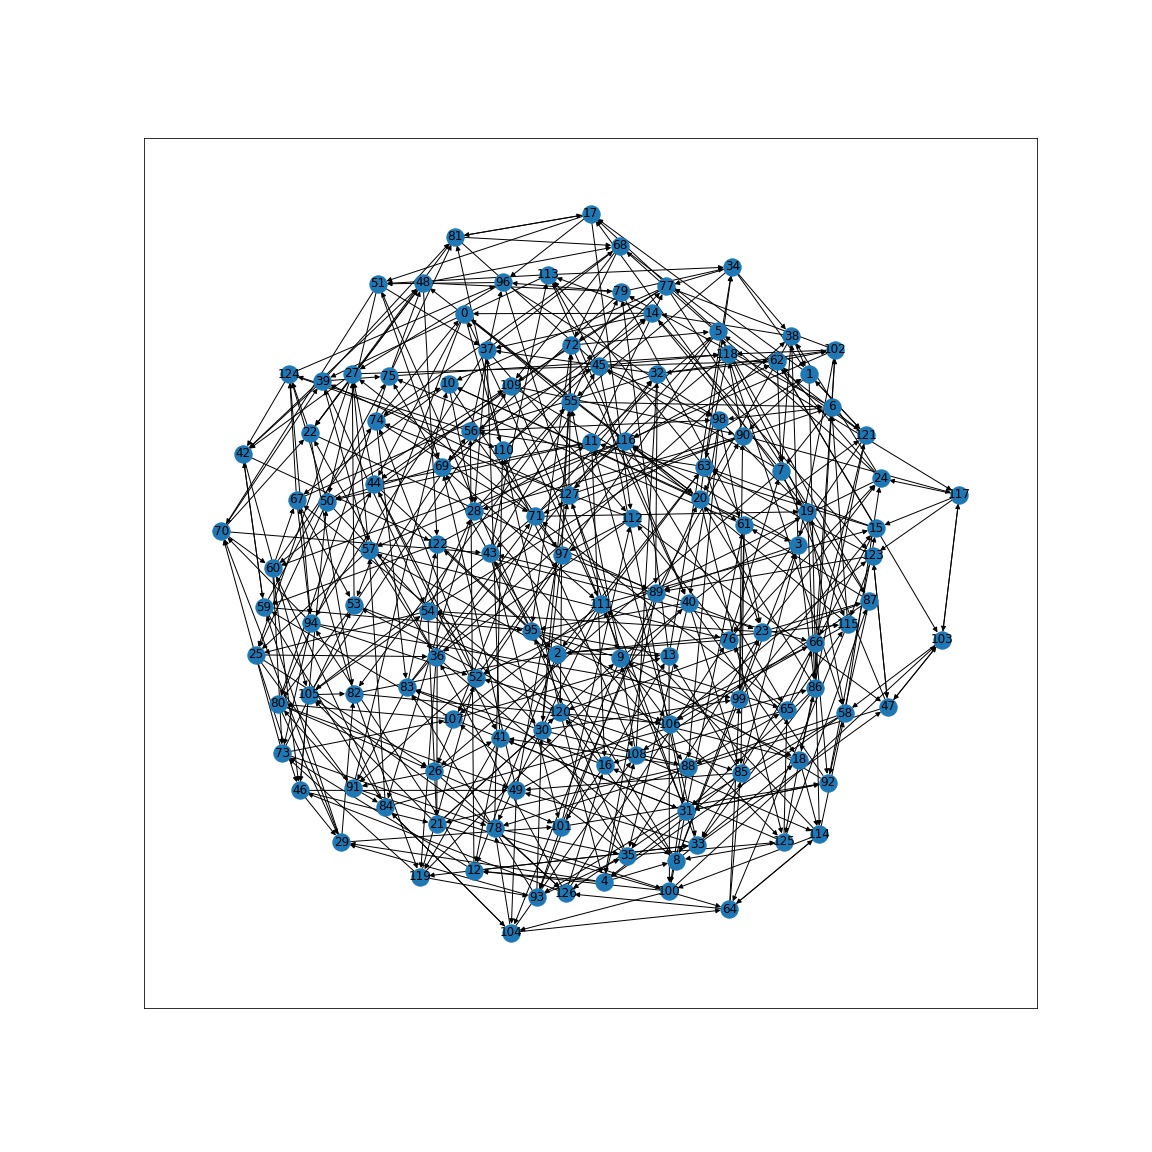}
\includegraphics[width=0.3\textwidth]{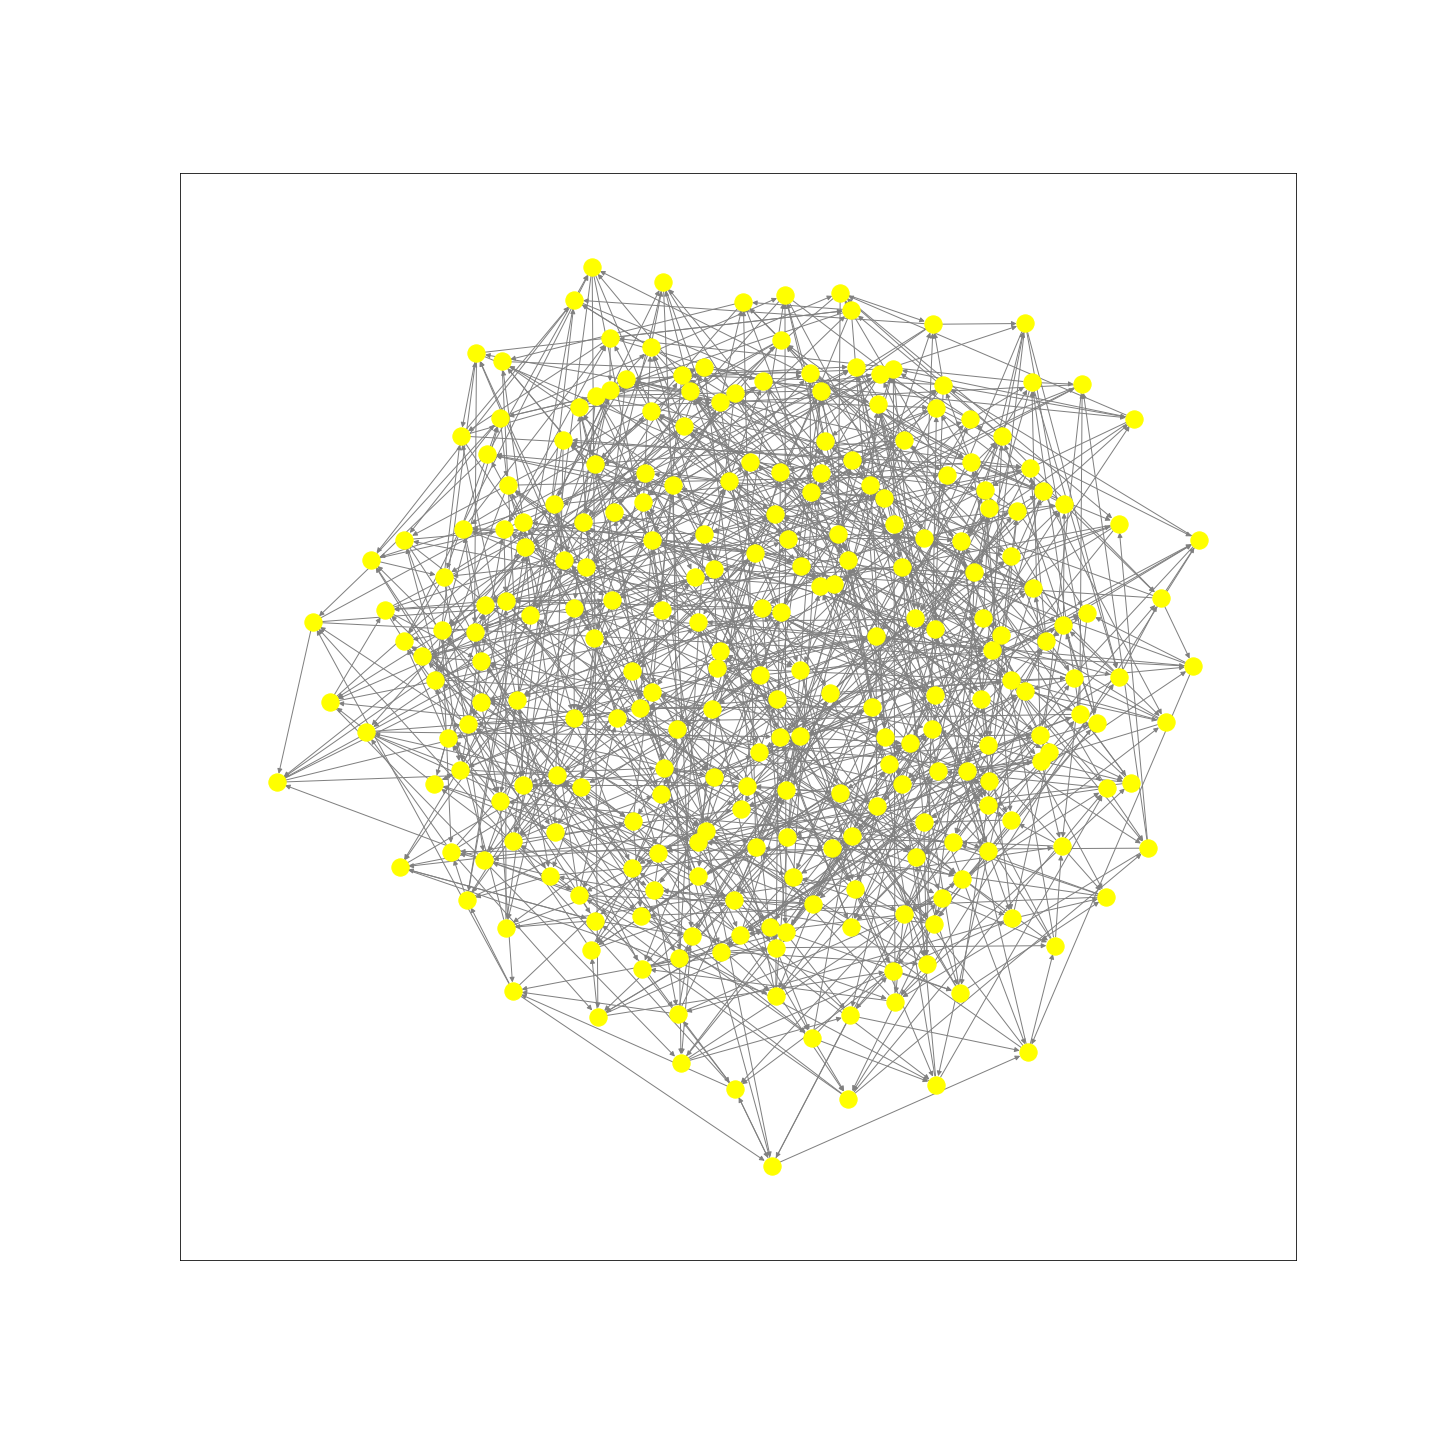}
\caption{Shortest path expander topologies generated by the incremental shortest path algorithm described in Section \ref{sec:incspath}: (a) $(N=64,k=4)$; (b) $(N=128,k=4)$; (c) $(N=256,k=4)$}
\label{fig:shortestpathtopo}
\end{figure*}

Minimizing the number of VCs to make a given set of routes deadlock free is NP-hard~\cite{Domke11}. The holy grail here of course is to perform joint route-finding and VC assignment. In this case, one needs to find routes that both yield near-optimal \ata performance and admit a layering scheme (with small number of layers) such that the resultant VC dependency graph has no cycles. This is a topic of future research for us. 

\section{Heuristics for generating good topologies}
\label{sec:incspath}

In this section, we describe a simple algorithmic heuristic inspired by the literature on ``network formation" that tends to generate topologies on $N$ nodes and degree $k$ that have good performance for the \texttt{alltoall} collective. The steps are described below.

\begin{enumerate}
\item Start from a weighted complete graph $G=(V,E,w)$ where $V = \{1,2,\ldots,N\}$, $E = V \times V$, and link weights $w:E\to \{\epsilon\}$, where $\epsilon$ is a small constant.
\item Iteratively lay down the shortest paths for each commodity $(s,d)$ one-by-one. After a shortest path $p$ is laid between $s$ and $d$, do the following:
\begin{enumerate}
\item Minimize congestion on existing links: Increment the link weights along the path $p$. Future commodities are unlikely to flow over such congested links unless they have no choice. 
\item Do not violate degree bounds: For all nodes $u\in V$ which now have more than $k$ links incident on it with $w > \epsilon$, then remove all the $\epsilon$-weighted links incident on $u$. 
\end{enumerate}
\item Repeat until all $N\times (N-1)$ commodities are routed
\item Return resultant graph $G$ which is $k$-regular. 
\end{enumerate}

We tested this algorithms for a few values of $N$ and $k$, and it produces expander like topologies. We refer to this family of graphs as \emph{shortest path expanders}. This is not surprising since every node tries to make connections with farther away nodes which obeying the degree constraints. Figure \ref{fig:shortestpathtopo} shows example degree 4 topologies on 64, 128, and 256 nodes. These are directed topologies that have similar or slightly better performance than the GenKautz graph and other expander graphs on the same parameters. This approach is promising since it can be adapted to generate bidirectional topologies as well. A more systematic evaluation of the performance of such topologies with respect to other expander graphs will occur in the near future.
